# Supplementary material for: Asymptotically optimal data analysis for rejecting local realism
Source: arXiv:1108.2468 ancillary file (2011-12-15)
Supplement: Supplementary file 1 [file user_guide.pdf]

# Local Realism Analysis Engine: User Guide

Yanbao Zhang

University of Colorado at Boulder and National Institute of Standards and Technology, Boulder, CO

Emanuel Knill, Scott Glancy

National Institute of Standards and Technology, Boulder, CO

## 1 Overview

The purpose of the Local Realism Analysis Engine (LRE) is to perform online and offline analysis of measurements obtained with randomly chosen measurement settings at two well-separated locations. The LRE determines the current and overall violation of local realism (LR). If LR is violated, it provides a measure of this violation in terms of the log- $p$ -value for violation. It is asymptotically optimal for independent measurements of identical states. If LR is not violated, it can provide feedback on the degree of nonviolation. This is accomplished by comparing the observed measurements to those that a reference or goal state would produce. The user must specify the goal state's probability distribution for measurement settings and outcomes that should be expected if the experiment is set up as intended. The motivation and theory for the LRE are described in [1].

This document gives a user-level specification of the LRE. The implementation of the LRE provided with this guide can be used with **Octave** or **Matlab**<sup>1</sup>. First we describe the state of the LRE. Then we define the functions that are used to initialize, modify and update the LRE state. Next we describe functions useful for supporting the LRE, such as functions to compute reference measurement distributions and calculate anticipated LR violation for standard experimental situations. Finally we give functions that can be used to simulate an experiment with the LRE. Examples of LRE usage are given for reference. For a quick start, one can go directly to Sec. 5. You may use, copy and distribute this software, provided that you keep intact the entire notice in Sec. 7

## 2 LRE State

The LRE state is characterized by experiment configuration, analysis and display variables, and the saved statistics of experimental data so far. Once the variables are initialized, the engine updates the state each time a new block of data is received. The state variables are maintained internally. From a user's perspective, they serve to formally define the state and behavior of the LRE and are therefore needed for fully understanding LRE dynamics. The state variables are controlled through functions and are not intended to be accessed or changed directly. We define them below as part of the LRE specification. In the implementation provided with this guide, they are accessible as global variables. Future implementations may choose to hide them, so the normal user should not rely on global access and use only the interface functions specified later.

### 2.1 Experimental Configuration

For the purposes of a test of LR, an experimental configuration is characterized by the number of measurement settings, their probability distribution, and the number of possible outcomes for a setting. These configuration variables are set when the LRE is initialized. Note that each block of data provided to the LRE must conform to the values of these parameters. The variables used by the LRE are:

**n\_settings\_a**, **n\_settings\_b**: The number of measurement settings available to Alice and Bob, respectively.

---

<sup>1</sup>The use of trade names is for informational purposes only and does not imply endorsement by NIST.

**n\_outcomes\_a, n\_outcomes\_b:** The number of possible measurement outcomes for each setting of Alice and Bob, respectively.

**p\_settings:** The joint probability distribution with which Alice and Bob choose their settings. This choice is assumed to be independent of the state being measured.

## 2.2 Analysis and Display Variables

For the purposes of analysis, a “data point” is the setting and outcome combination that is used and observed in one trial of the experiment. A “data block” consists of a number of data points.

The main task of the LRE on receiving a new block of data is to update the log- $p$ -values **test\_lp\_total**, **test\_lp** and **goal\_lp**. (We define the log- $p$ -value to be  $-\log_2(p)$ , where  $p$  is the  $p$ -value as computed according to our algorithm.) While **test\_lp\_total** is the overall log- $p$ -value reported after a completed experiment, the log- $p$ -values **test\_lp** and **goal\_lp** help for monitoring the experimental progress. A positive value of **test\_lp** is sufficient for LR violation. If the experiment is stable, it is also asymptotically necessary. Negative values of **test\_lp** are not informative<sup>2</sup>. The value of **goal\_lp** reflects how well we are doing in approaching a specified goal distribution for settings and outcomes and can be used to tweak an experiment when there is no violation of LR. (When there is no violation, **test\_lp** is near zero and insensitive to tweaks.) A goal of tweaking the experiment can be to increase **goal\_lp**. Its use is explained in the example in Sec. 5.2.

In order for these log- $p$ -values to be useful during an experiment, they need to adapt to changes in the experimental state. The amount of data that plays a role is controlled via data “half-lives”. Roughly, these half-lives control how many of the last data points are used in computing and updating the log- $p$ -values. We use half-lives instead of data windows so that we can avoid storing old data. As a result, the contribution of data points decays exponentially as more data is acquired.

The relevant part of the LRE state is described by the following variables.

**goal\_frequencies:** This describes the frequencies of settings and outcomes for a goal state. To be useful, it should be possible to realistically approach them in the experiment, and they should violate LR. We provide functions to compute them for some typical experimental configurations. It is not a good idea (and probably not realistic) to have any of the goal state’s frequencies be zero. If the corresponding settings and outcomes occur in the experiment, then **goal\_lp** can become  $-\infty$ , and, without intervention, will stay there.

When **goal\_frequencies** is set or updated, the LRE computes the following:

**goal\_sd:** The statistical strength of the goal frequencies for rejection of LR. If the experimental state achieves the goal frequencies, then **goal\_lp** should approach the value of **goal\_sd** multiplied by the effective number of trials according to **goal\_lp\_weight\_snumber** (defined below).

**goal\_ratios:** The computation of **goal\_lp** requires probability ratios as described in [1]. This variable contains the needed ratios.

**data\_half\_life:** The LRE maintains cumulative setting and outcome frequencies. Each data point contributes to the cumulative frequencies with a weight that decays over time. The idea is that a data point’s weight should be 1/2 of the most recent point’s weight after **data\_half\_life** more points have been acquired. The calculation takes into account that there are only finitely many data points so far but ensures that the ratio of weights for data points in successive blocks is the one expected in the asymptotic case. For simplicity, data points in the same block get the same weight. The details of the calculation are given in Sec. 6. To help with this calculation the LRE computes and updates the following:

**data\_weight:** The weight used for the most recent data point contributing to the stored setting and outcome frequencies, **test\_frequencies**.

---

<sup>2</sup>We allow the log- $p$ -values to be negative for the purpose of tweaking an experiment. That is, we set the  $p$ -value equal to  $(\prod_{k=1}^n R_{k-1}(x_k))^{-1}$  and do not truncate it at 1, see [1].

**lp\_half\_life:** The effective half-life for computing **test\_lp** and **goal\_lp** can be set independently of **data\_half\_life**. The interpretation of **lp\_half\_life** differs from that of **data\_half\_life**. This is because the log-*p*-values are weighted sums of logarithms of probability ratios such as **goal\_ratios**, but not averages. In order to interpret the log-*p*-values as intended, the weights have a maximum value of 1, see Sec. 6 for an explanation. To calculate updated weights, the LRE computes and updates the following:

**test\_lp\_weight\_snumber, goal\_lp\_weight\_snumber:** Effective numbers of data points contributing to the computation of **test\_lp** and **goal\_lp**, respectively. These numbers are computed based on **lp\_half\_life** and the numbers of data points that have contributed to the respective log-*p*-value calculations. The log-*p*-values **test\_lp** and **goal\_lp** are updated accordingly.

**test\_lp\_data\_weight, goal\_lp\_data\_weight:** The weights of the most recent data points according to **lp\_half\_life** for updating **test\_lp\_weight\_snumber** and **goal\_lp\_weight\_snumber**, respectively.

**test\_lp\_tolerance:** The log-*p*-values for LR rejection based on the data (e.g., **test\_lp**) may be underestimated by a maximum of **test\_lp\_tolerance** per data point. The underestimate accounts for the possibility that the computation of optimal LR models may not reach the exact optima after the stopping criteria are satisfied. The value of **test\_lp\_tolerance** must be significantly smaller than the achieved log-*p*-value per data point violation in the experiment. Thus, if  $10^3$  trials are needed before violation is apparent, **test\_lp\_tolerance** should be much less than  $10^{-3}$ . Otherwise log-*p*-values may accumulate negative values. The default value of **test\_lp\_tolerance** is  $10^{-6}$ . Setting it significantly higher may speed up updates. See the last section of the appendix of [1] for the details.

## 2.3 Data Dependent Variables

**test\_frequencies:** The cumulative, weighted frequencies of experimental settings and outcomes.

**data\_weight:** The weight of the most recent data point contributing to **test\_frequencies**.

**num\_exps:** The total number of trials since the LRE was last reset.

**weight\_snumber:** The effective number of data points contributing to **test\_frequencies**.

**pred\_ratios:** The prediction-based probability ratios that will be used to update **test\_lp** and **test\_lp\_total** when the next block of data arrives. They are determined as explained in [1]. The estimated probability distribution in the numerator is derived from **test\_frequencies** by a maximum likelihood method to enforce the setting distribution and (if desired) the no-signaling constraints. Then, to avoid the possibility of getting stuck with log-*p*-values of  $-\infty$ , the distribution is modified by mixing in the setting-conditional uniform distribution, with weight  $1/(1+\text{weight\_snumber})$ .

**lr\_use\_cm:** This option variable controls whether to enforce no-signaling (also called “consistent marginals”) constraints when computing **pred\_ratios**. Its default value is 0 (false). Turning this option on can slow down updates but helps to reduce the log-*p*-value offset caused by the learning transient, when the number of data points is still small.

**test\_sd:** The statistical strength of rejection of LR of the estimated probability distribution used to generate **pred\_ratios**.

**test\_lp, goal\_lp:** The current log-*p*-values as described above. These are weighted according to **lp\_half\_life**.

**test\_lp\_weight\_snumber, goal\_lp\_weight\_snumber:** Effective numbers of data points contributing to the computation of **test\_lp** and **goal\_lp**, respectively.

**test\_lp\_total:** The total log-*p*-value for LR rejection since the last reset. Its value is the one that **test\_lp** would have if **lp\_half\_life** were infinity. This log-*p*-value should be reported as the overall log-*p*-value when analyzing data from a completed experiment.

`test_lp_v`, `goal_lp_v` and `test_lp_total_v`: Estimated variances of the `test_lp`, `goal_lp` and `test_lp_total`. When reporting `test_lp_total`, one can give the square root of `test_lp_total_v` as its standard error when giving it as a quantitative measure of success of the experiment. The other two variances can be used to assess the expected fluctuations in the corresponding log- $p$ -values when tweaking the experiment.

`test_sd2`, `goal_sd2`: The predicted variances of the log- $p$ -value increments at the next trial, calculated based on `pred_ratios` and `goal_ratios` respectively. These are internal variables needed to update the estimated variances.

### 3 LRE Interface

The specification of the LRE interface functions given here includes explicit instructions for calculating nominally inaccessible state variables and other internal parameters. The calculations need not be performed exactly as described here, as long as the specified behavior is preserved.

> `function lr_init(n_settings_a, n_settings_b, n_outcomes_a, n_outcomes_b, p_settings)`

Initialize the LRE. The arguments are

`n_settings_a`, `n_settings_b`: Positive integers giving the number of measurement settings of Alice and Bob, respectively.

`n_outcomes_a`, `n_outcomes_b`: Positive integers giving the number of outcomes of each setting of Alice and Bob, respectively.

`p_settings`: A column vector of dimension `n_settings_a * n_settings_b` giving the joint probability distribution for the settings used by Alice and Bob. The probability that Alice and Bob measure the  $k$ 'th and  $l$ 'th setting respectively is given by the  $k+(l-1)*n\_settings\_a$ 'th entry of the vector. This argument is optional and defaults to the uniform distribution.

After `lr_init` is called, the state of the LRE satisfies the following:

- The experimental configuration variables are set according to the arguments.
- `goal_frequencies`, `goal_sd`, `goal_sd2`, `test_frequencies`, `test_sd` and `test_sd2` are set to an undefined value (the empty vector []).
- `data_half_life` and `lp_half_life` are set to `Inf`.
- `num_exps`, `weight_snumber`, `goal_lp_weight_snumber`, `test_lp_weight_snumber`, `data_weight`, `test_lp_data_weight`, `goal_lp_data_weight`, `goal_lp`, `test_lp`, `test_lp_total`, `goal_lp_v`, `test_lp_v` and `test_lp_total_v` are set to 0.
- The ratios in `goal_ratios` and `pred_ratios` are set to 1.

> `function lr_set_tolerance(tolerance)`

Set the variable `test_lp_tolerance` to `tolerance`. This can be changed any time. It should be much less than the predicted violation `test_sd`, when this is clearly positive.

> `function lr_set_use_cm(t_or_f)`

Set the variable `lr_use_cm` to 1 (true) or 0 (false), which determines whether the no-signaling constraints are used in optimizations. The argument is boolean.

> `function lr_prime(frequencies_or_block, num)`

Prime the LRE with initial frequencies. The arguments are

`frequencies_or_block`: The frequencies of settings and outcomes of a block of data, or the block of data itself, as specified below.

**num**: If the first argument gives the frequencies, then this argument gives the number of data points that contribute to the frequencies. The argument **num** is optional. If it is given, the first argument must be a frequency array, not a block of data.

A block of data consists of a **num** by 4 matrix. Each row contains a specific data point, specified by four non-negative integers in the following order: Alice's setting, Alice's measurement outcome, Bob's setting, Bob's measurement outcome. The integers must be in the appropriate range. For example, Alice's settings must be between 1 and **n\_settings\_a**, and her outcomes must be between 0 and **n\_outcomes\_a-1**.

Frequencies are entered as an array of dimension **n\_settings\_a \* n\_settings\_b** by **n\_outcomes\_a \* n\_outcomes\_b**. The entry indexed by  $(k+(l-1)*n\_settings\_a, 1+r+s*n\_outcomes\_a)$  is the frequency with which Alice's (Bob's) outcome is **r** (**s**) for the setting indexed by **k** (**l**). The frequencies are normalized so that `sum(sum(frequencies)) = 1`.

The function **lr\_prime** assumes that the LRE has been initialized. It performs the following actions:

- The LRE state is reset via **lr\_reset()** (specified below).
- Let **bf** be the setting and outcome frequencies computed (if necessary) from the input, and let **n** be the number of data points that contribute to these frequencies.
- Perform the following assignments:

```
num_exps = n;
data_weight = 1/n;
weight_snumber = n;
test_frequencies = bf;
```

- Use **test\_frequencies** to estimate the probabilities **fbf** of future settings and outcomes. Our implementation is equivalent to computing **fbf** in three steps. The first is to modify **bf** so that it has the correct setting distribution. The modification is equivalent to a maximum likelihood estimate with the setting distribution as a constraint. If **lr\_use\_cm** is 1 (true), the next step is to obtain the maximum likelihood estimate subject to the no-signaling constraints. The last step adjusts the estimate by mixing in the setting-conditional uniform distribution with weight  $1/(1+weight\_snumber)$ . Future implementations may perform this estimate differently.
- Let **lf** be the optimal LR frequencies witnessing the statistical strength of **fbf**. Compute the statistical strength **test\_sd** of **fbf** for rejection of LR according to  $test\_sd = \sum(\sum(fbf .* \log2(fbf./lf)))$ . The predicted variance is computed as  $test\_sd2 = \sum(\sum(fbf .* \log2(fbf./lf).^2)) - test\_sd^2$ .
- Set **pred\_ratios** = **fbf./lf**. We multiply **pred\_ratios** by a factor slightly smaller than 1 to account for not having found the exact optimal LR frequencies due to the optimization stopping criterion **test\_lp\_tolerance**, see [1] for details.
- If **goal\_frequencies** is defined, compute the initial values of **goal\_lp** and **goal\_lp\_v**, and set **goal\_lp\_data\_weight** = 1/n and **goal\_lp\_weight\_snumber** = n. The initial values of **goal\_lp** and **goal\_lp\_v** are given by  $\sum(\sum(n * bf .* \log2(goal\_ratios)))$  and  $n * goal\_sd2$ , respectively. See function **lr\_set\_goal** below for how **goal\_ratios** and the initial **goal\_sd2** are calculated. Finally, update **goal\_sd2** by setting  $goal\_sd2 = \sum(\sum(fbf .* \log2(goal\_ratios).^2)) - \sum(\sum(fbf .* \log2(goal\_ratios)))^2$ .

> **function lr\_update(frequencies\_or\_block, num)**

Update the LRE state according to new data. The arguments are as for the function **lr\_prime**. If **test\_frequencies** is undefined, **lr\_prime(frequencies\_or\_block, num)** is called. Otherwise the following actions are taken:

- Let **bf** be the setting and outcome frequencies computed (if necessary) from the input, and let **n** be the number of data points that contribute to these frequencies.

- Compute the weight `ndw` of the contribution of each new data point to `test_frequencies`. After computing `ndw`, `test_frequencies` is updated according to

$$\text{test\_frequencies} = (1 - \text{n*ndw}) * \text{test\_frequencies} + \text{n*ndw} * \text{bf};$$

To compute `ndw`, solve the equation

$$(1 - \text{n*ndw}) * \text{data\_weight} / \text{ndw} = 2^{(-\text{n}/\text{data\_half\_life})};$$

The formula is explained in Sec. 6. For constant block size `n` and no change in `data_half_life`, this ensures that the weight of the contribution of each data point in the `data_half_life/n`'th last block to `test_frequencies` is 1/2 of the weight of the most recent data point.

- Compute the new effective number of data points `ndwsn` as follows:

$$\text{ndwsn} = ((1 - \text{n*ndw})^2 / \text{weight\_snumber} + \text{n*ndw}^2)^{-1};$$

See Sec. 6 for an explanation.

- To update `test_lp` do the following:

- + Calculate the log-*p*-value increment `lpi` with respect to `pred_ratios` for the block of data:

$$\begin{aligned} \text{lpi} &= \text{sum}(\text{sum}(\text{n} * \text{bf} .* \log_2(\text{pred\_ratios}))); \\ \text{test\_lp\_total} &= \text{test\_lp\_total} + \text{lpi}; \\ \text{test\_lp\_total\_v} &= \text{test\_lp\_total\_v} + \text{test\_sd2} * \text{n} \end{aligned}$$

- + Compute `tlp_ndw` and `tlp_ndwsn` by following the steps used to compute `ndw` and `ndwsn`, using `test_lp_data_weight`, `test_lp_weight_snumber` and `lp_half_life` instead of `data_weight`, `data_weight_snumber` and `data_half_life`, respectively.

- + Obtain `tlpw` by solving

$$\text{tlp\_ndwsn} = (1 - \text{tlpw}) * \text{test\_lp\_weight\_snumber} + \text{n};$$

(If `test_lp_weight_snumber` is zero, set `tlpw` = 1.)

- + Set `test_lp` =  $(1 - \text{tlpw}) * \text{test\_lp} + \text{lpi}$ . This ensures that the weight of each data-point's contribution to the log-*p*-value is at most 1, necessary for interpreting `test_lp` as a valid log-*p*-value, see Sec. 6. It also ensures that the sum of the weights is `tlp_ndwsn`, so that `tlp_ndwsn` is the effective number of contributing data points consistent with the value of `lp_half_life`.

- + Set `test_lp_v` =  $(1 - \text{tlpw})^2 * \text{test\_lp\_v} + \text{test\_sd2} * \text{n}$ .

- Update `test_sd`, `test_sd2` and `pred_ratios` as explained in the description of the function `lr_prime`.
- If `goal_frequencies` is defined, first calculate the log-*p*-value increment `lpi_g` from `goal_ratios`, using the method for calculating `lpi` from `pred_ratios`. Then update `goal_lp` and `goal_lp_v` by following the steps used to update `test_lp` and `test_lp_v`, respectively. After that, update `goal_sd2` as in the function `lr_prime`.
- Complete the update by setting

$$\begin{aligned} \text{num\_exps} &= \text{num\_exps} + \text{n}; \\ \text{data\_weight} &= \text{ndw}; \text{weight\_snumber} = \text{ndwsn}; \\ \text{test\_lp\_data\_weight} &= \text{tlp\_ndw}; \text{test\_lp\_weight\_snumber} = \text{tlp\_ndwsn}; \end{aligned}$$

If `goal_frequencies` is defined, update `goal_lp_data_weight` and `goal_lp_weight_snumber` similarly.

```
> function lr_std_analysis(all_trials, verbose)
```

Run a full analysis of a complete data set using recommended parameters. The argument `all_trials` has the same form as a block of data. `verbose` is a boolean variable 1 or 0 indicating whether to print progress information during the analysis. This argument is optional and defaults to 1. The function returns the value of `test_lp_total` and the square root of `test_lp_total_v`, which is the estimated standard error of `test_lp_total` with respect to its mean for repetitions of the same experiment.

Let `num` be the number of trials as indicated by the number of rows in `all_trials`. Let `so_num` be the number of possible setting and outcome combinations, `n_settings_a * n_settings_b * n_outcomes_a * n_outcomes_b`. Our implementation of the function `lr_std_analysis` does the following after re-setting the LRE:

- Set `lr_use_cm = 1` and `test_lp_tolerance = min(1E-6, 1/(num*100))`.
- Set `block_size = ceil(max(num/1000, so_num * log(2*so_num)))` as recommended in [1].
- Apply the function `lr_update` to consecutive blocks of `block_size` rows of `all_trials`. The last block may be smaller if `block_size` does not divide `num`.
- Return `test_lp_total` and the square root of `test_lp_total_v`.

```
> function lr_set_goal(frequencies)
```

(Re)set the variable `goal_frequencies` to the argument `frequencies`, and (re)compute the value of the statistical strength `goal_sd`, the predicted variance `goal_sd2` and the probability ratios `goal_ratios`. The computations of `goal_sd`, `goal_sd2` and `goal_ratios` are performed like those of `test_sd`, `test_sd2` and `pred_ratios` respectively (see function `lr_prime`), but instead of the estimated probability distribution `fbf` the computations use `frequencies`. Note that, if `goal_frequencies` is (re)set after priming the LRE, then `goal_sd2` is updated in the same way as in the function `lr_prime`. The log-*p*-value `goal_lp` and the associated variables `goal_lp_data_weight` and `goal_lp_weight_snumber` are unchanged. This means that the old value of `goal_frequencies` continues contributing to `goal_lp` via the data added before this function was called. This contribution decays according to the relevant half-life `lp_half_life`.

Note: If the function `lr_prime` is used as a way to reduce the learning transient by initializing `pred_ratios` with prior knowledge from theory or earlier experiments such as tomography experiments, it is a good idea to delay setting the goal frequencies until after priming. This makes sure that `goal_lp` remains zero until the experiment starts properly.

```
> function lr_set_data_half_life(half_life)
```

Set `data_half_life = half_life`. Contributions to frequencies from old and new data decay at this rate from now on. Relative weights within old data are unchanged.

```
> function lr_set_lp_half_life(half_life)
```

Set `lp_half_life = half_life`. Contributions to log-*p*-values from old and new data decay at this rate from now on. Relative weights within contributions from old data are unchanged.

```
> function lr_reset()
```

Reset the state of the LRE. Only the data-independent variables are kept. That is, the state is the same as after

```
g = goal_frequencies; dh = data_half_life; lh = lp_half_life;
lr_init(n_settings_a, n_settings_b, n_outcomes_a, n_outcomes_b, p_settings);
lr_set_goal(g); lr_set_data_half_life(dh); lr_set_lp_half_life(lh);
```

`test_lp_tolerance` and `lr_use_cm` are unchanged by the function `lr_reset`.

```
> function lr_lps()
```

Return `goal_lp`, `test_lp`, and `test_lp_total`.

```

> function lr_lp_vs()
    Return goal_lp_v, test_lp_v, and test_lp_total_v.

> function lr_sds()
    Return goal_sd and test_sd.

> function lr_snumbers()
    Return weight_snumber, goal_lp_weight_snumber, and test_lp_weight_snumber.

```

## 4 LRE Support Functions

By setting the half-lives to infinity, the LRE can be used directly to analyze existing data for violation of LR. If one can make a *blind* prediction of the frequencies of settings and outcomes, then they can be used to prime the engine and get better log- $p$ -values less affected by having to learn the setting and outcome frequencies from the initial blocks of data.

One of the applications of the LRE is to monitor an ongoing experiment, even if the data are not currently in a region where LR is violated. For this we provide functions to compute realistic goal frequencies associated with goal states and (possibly optimized) measurement settings. With the goal frequencies, monitoring `goal_lp` may help to tweak the experiment toward LR violation. Once LR is violated, one can try to improve `test_lp` directly, without necessarily moving the experiment to the hoped-for goal.

The LRE support functions enable computing goal frequencies and their statistical strengths for rejecting LR, given experimental settings and noise parameters. They also make it possible to generate simulated data to test and explore LRE functions. The support function arguments include a state specification, `state_spec`; a noise specification (losses and visibility), `noise_spec`; and a measurement setting specification, `settings_spec`.

**state\_spec**: State specification. Currently only balanced and unbalanced Bell states as if prepared by idealized down-conversion can be specified. For this case, `state_spec` is a two-component vector, specifying the bias  $\theta$  and population  $p$  of the state given by

$$|\psi\rangle = \sqrt{1-p}|0\rangle_A|0\rangle_B + \sqrt{p}(\sin(\theta)|H\rangle_A|H\rangle_B + \cos(\theta)|V\rangle_A|V\rangle_B). \quad (1)$$

We assume that double and higher-order pair emission is negligible. Forms of `state_spec` with more than two components are reserved for other types of states.

**noise\_spec**: Noise specification. For the case of experiments involving the states in Eq. (1) (as indicated by `state_spec` being a vector of length 2), there are up to three parameters: losses  $\eta_a$  and  $\eta_b$  for Alice and Bob, and visibility  $v$ . If `noise_spec` is a real number, it specifies the two identical losses, and visibility defaults to 1. If `noise_spec` is a vector of length 2, the first entry is  $\eta_a = \eta_b$ , and the second is the visibility. If it is a vector of length 3, it contains  $\eta_a$ ,  $\eta_b$  and  $v$ , in this order.

**settings\_spec**: Description of Alice’s and Bob’s measurement configurations. For Bell-type experiments, this is a cell array with the following components:

- **settings\_spec{1}**: The numbers of settings available to Alice and Bob. If `length(settings_spec{1}) == 0`, they default to 2. If `length(settings_spec{1}) == 1`, then both numbers of settings are given by `settings_spec{1}`. If `length(settings_spec{1}) == 2`, then Alice’s and Bob’s numbers of settings are the first and second entries, respectively.
- **settings\_spec{2}**: The numbers of measurement outcomes (setting-independent) for Alice and Bob. If `length(settings_spec{2}) == 0`, they default to 2. Otherwise, they are treated like `settings_spec{1}`. For experiments involving the states in Eq. (1), only the values 2 and 3 make sense. The measurement settings are specified by observables with eigenvalues  $+1, -1$  (see the description of `settings_spec{4}`). The  $+1$ -eigenvalue outcomes are assigned to outcome 1, when entered in data for the LRE. If `settings_spec{2} == 2`, we assume that there is only one detector, and it “clicks” if the photon is found in the  $+1$ -eigenvalue eigenstate. Otherwise we don’t



detect the photon (it is lost, or it would have been found in the  $-1$ -eigenvalue eigenstate), which is assigned to outcome 0. If `settings_spec{2} == 3`, we assume that there are two detectors, one for each eigenvalue. The  $+1$  and  $-1$  eigenvalues are assigned to outcomes 1 and 2, respectively. No detection is assigned to 0.

- `settings_spec{3}`: The probability distribution of the measurement setting choices. If `length(settings_spec{3}) == 0`, it is assumed to be uniform. Otherwise it has the same form as `p_settings`.
- `settings_spec{4}`: Alice's measurement settings. This is a `n_settings_a` by 1 or 2 matrix. The  $k$ 'th setting is given by its  $k$ 'th row. It specifies angles for the Jones vector of the polarization  $+1$ -eigenstate of the measurement operator mentioned above. If there is only one parameter  $\theta$ , the Jones vector is  $(\cos(\theta), \sin(\theta))$ , indicating polarization at angle  $\theta$  from horizontal polarization. If there are two parameters  $\theta$  and  $\phi$ , the Jones vector is  $(\cos(\theta), e^{i\phi} \sin(\theta))$ . The vectors can be interpreted as photon polarization states with  $(0, 1)$ ,  $(1, 0)$ ,  $(1, 1)/\sqrt{2}$ , and  $(1 - i, 1 + i)/2$  the vertically, horizontally, diagonally and right-circularly polarized states, respectively.
- `settings_spec{5}`: Bob's measurement settings, in the same form as Alice's but with `n_settings_b` many rows.

The following functions are provided:

- ```
> function lr_config_freqs(state_spec, noise_spec, settings_spec)
```
- Return the probabilities of settings and outcomes according to the given experimental configuration. These probabilities are predicted by quantum theory. The returned value's data type is the same as that of `goal_frequencies` and the argument for the function `lr_set_goal`.
- ```
> function lr_config_analysis(state_spec, noise_spec, settings_spec)
```
- Analyze the given experimental configuration for violation of LR. The function returns `sd`, `frequencies`, `ratios`, `p_settings`, and `lr_frequencies`.
- `sd`: The statistical strength of the configuration for rejecting LR.
- `frequencies`: The quantum predicted frequencies of settings and outcomes. The data type matches that of `goal_frequencies`.
- `ratios`: The probability ratios for computing log- $p$ -values. The data type matches that of `goal_ratios`.
- `p_settings`: The probability distribution of settings inferred from the arguments.
- `lr_frequencies`: The frequencies of settings and outcomes according to the optimal LR model. The data type is the same as that of `goal_frequencies`.
- ```
> function lr_config_optim(state_spec, noise_spec, settings_spec)
```
- Optimize the measurement settings for a specified experimental configuration by maximizing the statistical strength of LR violation. The optimization uses the given measurement settings as an initial point. A local optimum is found. The function returns `opt_settings` and `opt_sd`, where
- `opt_settings`: The locally optimal settings found in the format matching the `settings_spec` argument. Only setting parameters of the argument are changed.
- `opt_sd`: The statistical strength for LR violation of the optimal settings.
- ```
> function lr_test_simulation(state_spec, noise_spec, settings_spec, num)
```
- Simulate `num` many trials according to the given experimental configuration. The function returns a block of data `data_block`, in the correct form for use as the `frequencies_or_block` argument in LRE update functions.

## 5 LRE Usage Examples

**Note:** The implementation of the LRE provided with this guide is “research grade”. It is inconsistently documented and should be considered unstable. It does not perform consistency checks on user-provided inputs. The following observation may help: Inconsistencies in user-provided input often result in array mismatch errors. If changes are made to the code, there is a minimal test suite (see `testsuite.m`) to perform a few simple (but incomplete) specification tests.

In the examples, the commands are shown without a prompt and are intended to be invoked in an `Octave` or `Matlab` shell. The LRE file `prep_lre.m` must be located on the path used to find scripts. Commands that are specific to this implementation of the LRE have comments starting with `%**`. Scripts for the examples are given with the code, see `example1.m` and `example2.m`.

### 5.1 Analyzing an Existing Data Set

Here is an example of how to use the LRE for analyzing a data set.

For the implementation provided with this guide, the first step is always to initialize the LRE. This sets up the needed paths and variables.

```
prep_lre;
%** CAUTION: This script defines the global variables used. Most of
%** them are explained in the description of LRE parameters and
%** states. There are some exceptions. Be aware of the possibility
%** of conflict if any of these variable names are used
%** elsewhere. Check pre_lre.m for the list of variable names.
```

Normally, one next loads the data set to be analyzed. For the purposes of this example, we simulate it by using the provided support functions. We assume that the measurement setting is chosen uniformly at random in each trial, the default.

```
sim_state_spec = [pi/4, 0.1];          % A Bell state, pair probability = 0.1.
sim_noise_spec = [0.95, 0.97];         % The efficiencies are 0.95, the visibility is 0.97.
sim_settings_spec = cell(5, 1);
sim_settings_spec{1} = 2;              % Two measurement settings each.
sim_settings_spec{2} = 3;              % Three outcomes for each setting.
sim_settings_spec{4} = [0; pi/4];      % Alice's settings, PBS angles.
sim_settings_spec{5} = [pi/8; -pi/8]; % Bob's settings, PBS angles.
[sd, frequencies] = lr_config_analysis(sim_state_spec, sim_noise_spec, sim_settings_spec);
disp(sd); % Expected statistical strength is sd = 0.0017331.
all_data = lr_test_simulation(sim_state_spec, sim_noise_spec, sim_settings_spec, 100000);
```

The first step of the analysis is to initialize the LRE.

```
lr_init(2, 2, 3, 3); % The arguments specify numbers of settings and outcomes.
```

The recommended method for analyzing data from a completed experiment is to use the provided function `lr_std_analysis` and report the returned value.

```
[violation_log_p_value, violation_log_p_value_sd] = lr_std_analysis(all_data);
% The final log-$p$-value is expected to be about 173 minus the learning
% transient, which we observed to be about 25 on average. The standard
% deviation of the reported log-$p$-value is around 20.
```

It may be desirable to choose some of the analysis parameters differently from the ones recommended in `lr_std_analysis`. If so, such a choice must be made *blindly*, that is before any information about the data to be analyzed is available. Information about the experiment before the data was acquired can be used. With such information, simulation may help in making better choices of analysis parameters.

Here is an instance of an explicit analysis with parameters chosen manually. First we reset the analysis engine.

```
lr_reset();
```

The main choice to be made is the number of data points in each block of data to be processed. It is necessary to make sure that the data in each block has a reasonable setting distribution. In particular, do not provide blocks with just one of the settings' data, otherwise the LRE estimated distributions may vary excessively, potentially worsening the log- $p$ -values.

Blocking the data improves efficiency, and having the first block be large enough to contain a good sample of the possible setting and outcome combinations mitigates the log- $p$ -value offset that typically arises from the learning transient. If the blocks are too large, we may reduce the log- $p$ -value by, in effect, not considering the first block for the log- $p$ -value calculations. The first block is used only to estimate the next block's setting and outcome frequencies. Thus, we recommend a block size of the larger of  $N/1000$ , where  $N$  is the number of trials, and  $d \ln(2d)$ , where  $d$  is the number of possible setting and outcome combinations. The first bound is chosen so that we do not lose too much significance by using the first block only for learning the setting and outcome distribution. The second ensures that if the setting and outcome distribution is uniform, the probability of having at least one event for each setting and outcome combination is at least  $1/2$ . For our example, the recommended block size is 154. For simplicity, we use 200.

Our implementation of the LRE has two parameters that affect the calculations of log- $p$ -values. The first is `test_lp_tolerance`, which affects the stopping criterion for the LR model optimization and the conservative factors used in `pred_ratios` and `goal_ratios` to ensure valid log- $p$ -values. It should be a small fraction of the anticipated statistical strength. If the strength is not particularly known, setting it to  $1/(100N)$  ensures that if the data has sufficient violation of LR, the stopping criterion does not significantly decrease the log- $p$ -value compared to what would be obtained with ideal LR model optimization. The second parameter is `lr_use_cm` and determines whether the no-signaling constraints are applied in estimating setting and outcome distributions. Applying these constraints increases computation time, but improves the estimates, particularly for the first few blocks.

```
lr_set_tolerance(1e-7); % 1/(100*N)
lr_use_cm = 1;          % Turn on "no-signaling" constraints.
```

If we have a reasonable estimate of the setting and outcome probability distribution that was obtained before the experiment was started, we can "prime" the LRE with these frequencies. This can reduce or eliminate the effect of the learning transient. If these frequencies are available in `predicted_frequencies` and the statistics of the prediction are as good as if we had inferred them from `support_number` many trials, then we can invoke the following before analyzing the experimental data (after removing the comment symbol):

```
% lr_prime(predicted_frequencies, support_number);
```

If the experiment was not stable for the entire time that it took to acquire the data, it may help to set the half-lives to values of the order of the stability time. This allows the LRE to adapt to drifts in the experimental state. Here we assume that the experiment was sufficiently stable and leave the half-lives at infinity, the default.

We now process one block of data at a time.

```
for i = 1:500
    lr_update(all_data(((i-1)*200+1):(i*200), 1:4));
    %** The following can be used to monitor progress:
    disp(sprintf('Log-p-value so far: %5.2f +/- %4.2f', test_lp_total, ...
        sqrt(test_lp_total_v)));
end
[glp, tlp, tlpt] = lr_lps();
disp(tlpt);          % The third value returned is the total
                    % log-$p$-value and the main result of the
                    % analysis.
[glpv, tlpv, tlptv] = lr_lp_vs();
disp(sqrt(tlptv));   % The third returned value is the variance of the total
                    % log-$p$-value.
```

## 5.2 Monitoring an Experiment in Progress

The following shows how one can use the LRE for monitoring an experiment in progress. The experiment to be simulated involves a (balanced) Bell state expected to be measured with 95% efficiency (all detectors). Measurements have three possible outcomes (two orthogonal polarizations and “no detection”). The setup aims for a photon-pair production probability of 0.1 and a visibility of 97%. The settings are intended to maximize the CHSH inequality. We begin with setting up the LRE environment.

```
prep_lre;
```

We initialize the LRE with two settings and three outcomes for each of Alice and Bob. The setting distribution is uniform, the default.

```
lr_init(2, 2, 3, 3);
```

For monitoring an experiment, it can be useful to set up ‘goal’ frequencies, which are the setting and outcome frequencies that can be realistically expected if the experiment is configured as intended. The goal frequencies are used by the LRE to calculate a quasi-log- $p$ -value, `goal_lp`. This behaves somewhat like the negative logarithm of a distance from the goal to the current experimental state: To approach the goal one tries to increase `goal_lp`. More negative values indicate that the current state is further from the goal.

By tweaking experimental parameters, one can aim for increasing `goal_lp`. If the goal state has been reached, then `goal_lp` is expected to be approximately the statistical strength of the goal frequencies times the effective number of contributing data points, `goal_lp_weight_snumber`. While monitoring `goal_lp`, one can also monitor `test_lp`. Unlike `goal_lp`, negative values of `test_lp` are not useful for tweaking. However, once `test_lp` becomes significantly positive, one can tweak it directly to optimize the experimental configuration. This allows exploring states that differ from the anticipated goal but may have better statistical strengths.

To set up the goal frequencies, we can use the support functions. We compute the goal frequencies based on reasonable and achievable state parameters.

```
state_spec = [pi/4, 0.1];           % Bell state with 0.1 probability of pairs.
noise_spec = [0.95, 0.97];         % Hoped-for efficiencies are 0.95, visibility is 0.97.
settings_spec = cell(5, 1);
settings_spec{1} = 2;               % Two settings each.
settings_spec{2} = 3;               % Three outcomes for each setting.
settings_spec{4} = [0; pi/4];       % Alice's settings, PBS angles.
settings_spec{5} = [pi/8; -pi/8];   % Bob's settings, PBS angles.
[sd, frequencies] = lr_config_analysis(state_spec, noise_spec, settings_spec);
disp(sd);
% The statistical strength for the goal frequencies is sd = 0.0017331.

% Set the goal frequencies in the LRE.
lr_set_goal(frequencies);
```

Next we set the half-lives for monitoring. It sets the time scale (in number of data points) after which data no longer contributes significantly to current statistics. The values should be a good multiple of the inverse of the expected statistical strength.

```
lr_set_data_half_life(4000);
lr_set_lp_half_life(4000);
```

For this example, we need to simulate the data, so we set up simulation parameters. For the purposes of the example, we assume that all is well except for the visibility, which is only 0.7 at the moment.

```
sim_state_spec = [pi/4, 0.1];
sim_noise_spec = [0.95, 0.7];      % Visibility is still low, at 0.7.
sim_settings_spec = settings_spec;
```

Normally we are not likely to know what the true experimental state parameters actually are. But for this example we do, so we can check whether we are going to violate LR, and we find that we are not.

```
[sd, frequencies] = lr_config_analysis(sim_state_spec, sim_noise_spec, sim_settings_spec);
disp(sd);
```

% Statistical strength is numerically 0, no violation.

This is how to get a block of 1000 data points.

```
data_block = lr_test_simulation(sim_state_spec, sim_noise_spec, sim_settings_spec, 1000);
```

```
% lr_use_cm = 1;    *** Turn on the "no-signaling" constraints for slightly
                    *** better predictions.
```

Run the experiment for a while.

```
lr_update(data_block);
for i = 1:20
    lr_update(lr_test_simulation(sim_state_spec, sim_noise_spec, sim_settings_spec, 1000));
    *** The following can be used to monitor progress:
    disp(sprintf('Block %2d, goal_lp:%5.2f +/- %4.2f, test_lp:%5.2f +/- %4.2f,...
        test_lp_total:%5.2f +/- %4.2f', i+1, goal_lp, sqrt(goal_lp_v), test_lp,...
        sqrt(test_lp_v), test_lp_total, sqrt(test_lp_total_v)));
end
```

We can check the status of the LRE by displaying the different statistics. See the explanation of the functions `lr_lps`, `lr_lp_vs`, `lr_sds` and `lr_snumbers`.

```
[glp, tlp, tlpt] = lr_lps(); disp([glp, tlp, tlpt]); % Log- $p$ -values
[glpv, tlpv, tlptv] = lr_lp_vs();
disp([glpv, tlpv, tlptv]); % Variances of the log- $p$ -values
[gsd, tsd] = lr_sds(); disp([gsd, tsd]); % Statistical strengths
[ws, gws, tws] = lr_snumbers(); disp([ws, gws, tws]); % Effective numbers of points
```

Suppose we tweak the experiment so that the visibility improves. Using our unrealistic knowledge of the true visibility, we can check the expected statistical strength.

```
sim_noise_spec=[0.95, 0.8];
[sd, frequencies] = lr_config_analysis(sim_state_spec, sim_noise_spec, sim_settings_spec);
disp(sd);
```

% Statistical strength is now  $1.5e-5$ .

Run the experiment for a while.

```
for i = 1:40
    lr_update(lr_test_simulation(sim_state_spec, sim_noise_spec, sim_settings_spec, 1000));
    *** The following can be used to monitor progress:
    disp(sprintf('Block %2d, goal_lp:%5.2f +/- %4.2f, test_lp:%5.2f +/- %4.2f,...
        test_lp_total:%5.2f +/- %4.2f', i+21, goal_lp, sqrt(goal_lp_v), test_lp,...
        sqrt(test_lp_v), test_lp_total, sqrt(test_lp_total_v)));
end
```

The half-lives were not set high enough to clearly see the violation yet. But the goal log- $p$ -value `goal_lp` should have increased noticeably, suggesting that we improved the experiment in a useful direction. We tweak it a bit more, in this case improving the visibility to that assumed for the goal frequencies, and continue running the experiment.

```

sim_noise_spec=[0.95, 0.97];
for i = 1:40
    lr_update(lr_test_simulation(sim_state_spec, sim_noise_spec, sim_settings_spec, 1000));
    %** The following can be used to monitor progress:
    disp(sprintf('Block %2d, goal_lp:%5.2f +/- %4.2f, test_lp:%5.2f +/- %4.2f,...
        test_lp_total:%5.2f +/- %4.2f', i+61, goal_lp, sqrt(goal_lp_v), test_lp,...
        sqrt(test_lp_v), test_lp_total, sqrt(test_lp_total_v)));
end

```

The violation should now be noticeable, with `test_lp` now positive.

## 6 Technical Notes

### 6.1 Data Half-lives and Data Weights

The LRE is designed to require minimal memory of past data. Online monitoring of experiments requires that only recently acquired data contributes significantly to the various statistics being tracked. This is made possible by updating the recorded setting and outcome frequencies by setting them to a convex combination of new and old frequencies. Let  $d_i$  be the  $i$ 'th data point represented by a 0/1-vector whose length is the number of setting and outcome combinations and that has a single 1 in the position corresponding to the  $i$ 'th setting and outcome combination. The frequency vector for all data points is given by  $\sum_{i=1}^N d_i/N$ , where  $N$  is the total number of data points. This is the final value of `test_frequencies` if `data_half_life = Inf`. In general, after the  $n$ 'th data point is acquired, the value of `test_frequencies` is given by a weighted combination  $f_n = \sum_{i=1}^n w_{n,i} d_i$ , where  $0 \leq w_{n,i} \leq 1$  and  $\sum_{i=1}^n w_{n,i} = 1$ . To minimize what we have to remember of the past, we wish to update the frequencies so that  $f_{n+1} = v_{n+1} d_{n+1} + (1 - v_{n+1}) f_n$ , where  $0 \leq v_{n+1} \leq 1$ . The quantity  $v_{n+1}$  is the weight of the  $(n+1)$ 'th data point after acquiring  $(n+1)$  data points. For efficiency and because there is little new information in individual data points, we prefer to update frequencies and other statistics one block of data at a time. Blocking does not affect the validity of the computed log- $p$ -values. We implement blocking by having the weights of data points within a block be identical. Let  $D_k$  be the sum of the  $d_i$  contributing to the  $k$ 'th block, and let  $m_k$  be the number of data points in the block. In terms of blocks, we use the frequency update  $F_{k+1} = V_{k+1} D_{k+1} + (1 - m_{k+1} V_{k+1}) F_k$ , with  $0 \leq V_{k+1} \leq 1/m_{k+1}$ . The interpretation of  $V_{k+1}$  is similar to  $v_{n+1}$  above, but it is the identical weight of each data point in the  $(k+1)$ 'th block. Its value is computed according to an approximate half-life  $\lambda$  (specified by the parameter `data_half_life`). For a normal geometric decay, this requires  $w_{n,i}/w_{n,i+1} = 2^{-1/\lambda}$ . Because we have blocked the data, matching the half life on average requires  $V_k(1 - m_{k+1} V_{k+1})/V_{k+1} = 2^{-m_{k+1}/\lambda}$  to get the right ratio of weights between the last two contributing blocks after the update. We solve this equation for  $V_{k+1}$  to get

$$V_{k+1} = \frac{V_k}{m_{k+1} V_k + 2^{-m_{k+1}/\lambda}}. \quad (2)$$

Thus the update requires keeping track of the weight of the most recent point, which after the update is given by  $V_{k+1}$ . The first block requires special treatment: We set  $V_1 = 1/m_1$ .

We use a similar geometrical weight strategy to update the log- $p$ -values. However, the contribution to the log- $p$ -value of the most recent data point should be weighted by 1, and the sum of the weights should be an effective number of contributing data points. To ensure that the interpretation of the weighted combination as a log- $p$ -value is valid, the weights must be between 0 and 1. The reason is as follows. As explained in [1], the starting point for computing a valid log- $p$ -value is that the ratio function  $R(x)$  (the value of variables such as `goal_ratios`) satisfies the two conditions  $0 \leq R(x)$  and  $\langle R(x) \rangle \leq 1$  for any LR model, where  $x$  is a trial's setting and outcome combination. Given such a function  $R(x)$ , if we modify it according to  $R'(x) = (R(x))^\gamma$  where  $0 \leq \gamma \leq 1$ , then  $0 \leq R'(x)$ , and for any LR model  $\langle R'(x) \rangle \leq \langle R(x) \rangle^\gamma \leq 1$  by concavity of the function  $y \rightarrow y^\gamma$ . Hence the log- $p$ -value computed using  $R'(x)$  instead of  $R(x)$  is also valid. In particular, the weighted combination of valid log- $p$ -value increments is a valid log- $p$ -value, if all weights are between 0 and 1.

One way to quantify an effective number of contributing data points is by noting that if we have independent instances  $r_i$  of a random variable  $R$  and estimate the mean according to weights  $w_{n,i}$  as  $\sum_i w_{n,i} r_i$ ,

the variance of the estimate is given by  $v_e = \sum_i w_{n,i}^2 v$ , where  $v$  is the variance of  $R$ . If the weights are all equal,  $v_e = v/n$ . For arbitrary weights,  $v_e = v/s_n$ , where  $s_n$  can be interpreted as an effective number of contributing points. Thus,  $s_n = 1/\sum_i w_{n,i}^2$ . Let  $S_k$  be the effective number of contributing points after the  $k$ 'th block has been received. To update  $S_k$  when it is nonzero, we use the following relationship implied by the formula for  $s_n$ :

$$\frac{1}{S_{k+1}} = m_{k+1}(V_{k+1})^2 + (1 - m_{k+1}V_{k+1})^2 \frac{1}{S_k}, \quad (3)$$

where  $V_{k+1}$  is given by Eq. (2).

We also account for the following issues: First, the first nonzero  $S_k$  depends on which effective number suffixed by `weight_snumber` it is. For `weight_snumber`,  $S_1 = m_1$ ; for `test_lp_weight_snumber`,  $S_1 = 0$  and  $S_2 = m_2$ ; and for `goal_lp_weight_snumber`, the  $S_k$  are nonzero only after the goal frequencies are set. Second, for different effective numbers, the weights of the most recent data points  $V_k$  are different. This is because the half-life for the log- $p$ -values can be different from the half-life for the setting and outcome frequencies, and because goal frequencies can be set anytime. Hence, we need to separately keep track of these weights with the variables suffixed by `data_weight`. Also, the weight  $V_k$  is nonzero only after the corresponding  $S_k$  is nonzero. If  $S_l$  is the first nonzero effective number, then  $V_i = 0$ ,  $i = 1, \dots, (l-1)$ , and  $V_l = 1/S_l$ . After that, the  $V_k$  are updated according to Eq. (2).

To see what to expect of the effective number of contributing data points given the half-life  $\lambda$ , consider the case of block size 1 in the asymptotic limit. Compute  $1/S_\infty = \sum_i (1-2^{-1/\lambda})^2 2^{-2i/\lambda} = (1-2^{-1/\lambda})/(1+2^{-1/\lambda})$ . For large  $\lambda$ ,  $S_\infty \approx (2/\ln(2))\lambda \approx 2.9\lambda$ .

Given the corresponding effective numbers of contributing data points, we compute and update the log- $p$ -values `test_lp` and `goal_lp` as follows. Consider the case for `test_lp`. Write  $L_k$  for the value of `test_lp` after the  $k$ 'th block of data has been processed. We compute  $L_{k+1}$  so that it is a weighted combination of  $L_k$  and the log- $p$ -value contributions from the last block of data, and the total weight of log- $p$ -value contributions is given by the corresponding  $S_{k+1}$ . Let  $B_k$  be the sum of the log- $p$ -value contributions of the data points in the  $k$ 'th block. Thus, we have  $L_{k+1} = B_{k+1} + W_{k+1}L_k$ , where  $W_{k+1}$  is obtained by solving  $m_{k+1} + W_{k+1}S_k = S_{k+1}$ . This ensures that  $0 \leq W_{k+1} \leq 1$ , so that the weight of the log- $p$ -value increment due to each data point is at most 1. Consequently,  $L_{k+1}$  is always a valid log- $p$ -value. We can use the same strategy to compute and update `goal_lp`.

## 7 Software Disclaimer

This research software ("the LRE") is provided by NIST as a public service. You may use, copy and distribute copies of the software in any medium, provided that you keep intact this entire notice. You may improve, modify and create derivative works of the software or any portion of the software, and you may copy and distribute such modifications or works. Modified works should carry a notice stating that you changed the software and should note the date and nature of any such change. Please explicitly acknowledge the National Institute of Standards and Technology as the source of the software.

The software is expressly provided "AS IS." NIST MAKES NO WARRANTY OF ANY KIND, EXPRESS, IMPLIED, IN FACT OR ARISING BY OPERATION OF LAW, INCLUDING, WITHOUT LIMITATION, THE IMPLIED WARRANTY OF MERCHANTABILITY, FITNESS FOR A PARTICULAR PURPOSE, NON-INFRINGEMENT AND DATA ACCURACY. NIST NEITHER REPRESENTS NOR WARRANTS THAT THE OPERATION OF THE SOFTWARE WILL BE UNINTERRUPTED OR ERROR-FREE, OR THAT ANY DEFECTS WILL BE CORRECTED. NIST DOES NOT WARRANT OR MAKE ANY REPRESENTATIONS REGARDING THE USE OF THE SOFTWARE OR THE RESULTS THEREOF, INCLUDING BUT NOT LIMITED TO THE CORRECTNESS, ACCURACY, RELIABILITY, OR USEFULNESS OF THE SOFTWARE.

You are solely responsible for determining the appropriateness of using and distributing the software and you assume all risks associated with its use, including but not limited to the risks and costs of program errors, compliance with applicable laws, damage to or loss of data, programs or equipment, and the unavailability or interruption of operation.

This software is not intended to be used in any situation where a failure could cause risk of injury or damage to property. The software and this documentation were developed by NIST employees. NIST employee contributions are not subject to copyright protection within the United States.

## References

- [1] Yanbao Zhang, Scott Glancy, and Emanuel Knill. Asymptotically optimal data analysis for rejecting local realism. As published, 2011.
